# Supplementary material for: Room-temperature vacancy emission from the jog on edge dislocation in FCC nickel under glide force
Source: arXiv:2411.00305 source file (2025-02-15)
Supplement: Supplementary file 1 [file Supplementary_Materials_250121.pdf]

# Supplementary materials of "Room-temperature vacancy emission from jog on edge dislocation in FCC nickel under glide force"

Yifan Wang[a,b,1], Wu-Rong Jian[a,1], Wei Cai[a,*]

[a] *Department of Mechanical Engineering, Stanford University, Stanford CA, 94305, USA*
[b] *Department of Materials Science and Engineering, Stanford University, Stanford CA, 94305, USA*

*January 21, 2025*

## 1. Procedure for generating jogged edge dislocation configuration

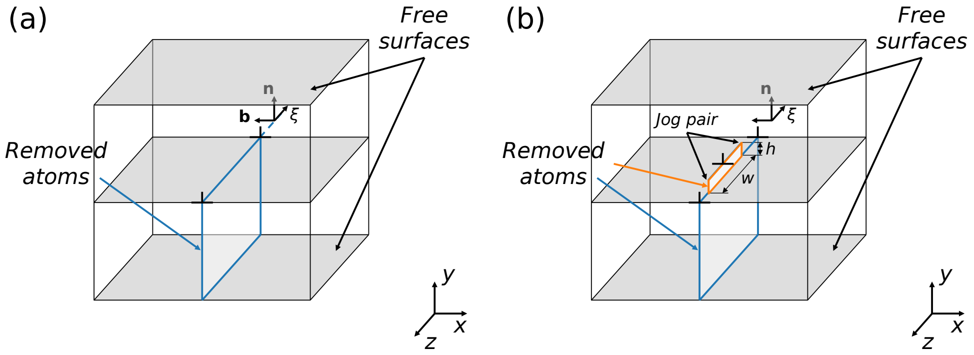


Figure 1: Schematic of the process for creating a unit jog pair on an edge dislocation in a single-crystal nickel with two free surfaces on the $y$-direction. (a) Edge dislocation without jog is created by removing one layer of atoms below the dislocation line. (b) Edge dislocation with a unit jog pair is created by an additional row of repeated atoms (orange region) above the slip plane with height of $h = \frac{1}{3}[111]$ and length $w = L_z/2$.

To construct the atomic configurations containing edge dislocations with and without jog, we first create an FCC single crystal nickel with the lattice

*Corresponding author
*Email address:* `caiwei@stanford.edu` (Wei Cai)
[1]Both authors contributed equally to the paper

constant of $a = 0.352\,\text{nm}$. The $x$-, $y$- and $z$-axes are aligned respectively along $[1\bar{1}0]$, $[111]$ and $[\bar{1}\bar{1}2]$ crystal orientations, with the simulation box dimension of $\sim (24 \times 15 \times 36)\,\text{nm}$ and about 1.16 million atoms. A single, straight-edge dislocation with line direction $\hat{\xi} = -\frac{1}{\sqrt{6}}[11\bar{2}]$ ($-\hat{z}$-direction) and $\mathbf{b} = -\frac{1}{2}[1\bar{1}0]$ ($-\hat{x}$-direction) is introduced by removing one layer of atoms below the dislocation slip plane. Two free-surfaces are created due to the lost of periodicity in the $y$-direction (slip-plane direction $\mathbf{n}$), as shown in Fig. 1(a). To build the jogged edge-dislocation configuration, we remove an additional row of atoms above the slip plane (orange region) with height of $h = \frac{1}{3}[111]$ and length $w = L_z/2$, as illustrated in Fig. 1(b). The result is a dislocation with a jog pair separated by a distance of half of the box length.

The resulting configurations are relaxed by energy minimization, which leads to the dissociated dislocation structure, as shown in Fig. 1 in the main text.

## 2. Dislocation velocity from displacement-time curves

To determine the velocity of dislocation as a function of applied stress, we extracted the dislocation displacement during the MD simulations in the gliding direction and plotted it as a function of time. We carry out the MD simulation for at least 200 ps (and up to 800 ps) to ensure the dislocation motion has reached steady-state for accurate determination of the velocity. We extract the velocity as the slope of the displacement-time curve using the second half of the simulation time. For intermediate applied stress, the dislocation motion becomes steady (constant velocity) after $\sim 10\,\text{ps}$, as shown in Fig. 2. Fig. 2(a) clearly shows the jog-dragging effect at $\tau = 100$ MPa, where the jogged dislocation has a lower velocity.

For jogged dislocations in the low-stress regime, we run the MD simulations for an extended time of 800 ps to make sure dislocation motion has reached steady-state. Fig. 3 shows that steady-state motion has been achieved in these simulations. For all the cases above 8 MPa, the dislocation displacement as a function of time during second half of the simulation can be fitted as a straight line with a $R^2 > 0.9$, further confirming steady-state motion. For the cases below 8 MPa, the jogged dislocation motion becomes jerky, because thermal activation is required, see Fig. 3 for the case of 5 MPa.

In the high-stress regime, the dislocation jog emits vacancies during motion. Due to periodic boundary conditions, the dislocation comes back to its previous location where it emitted the vacancy. To ensure that the

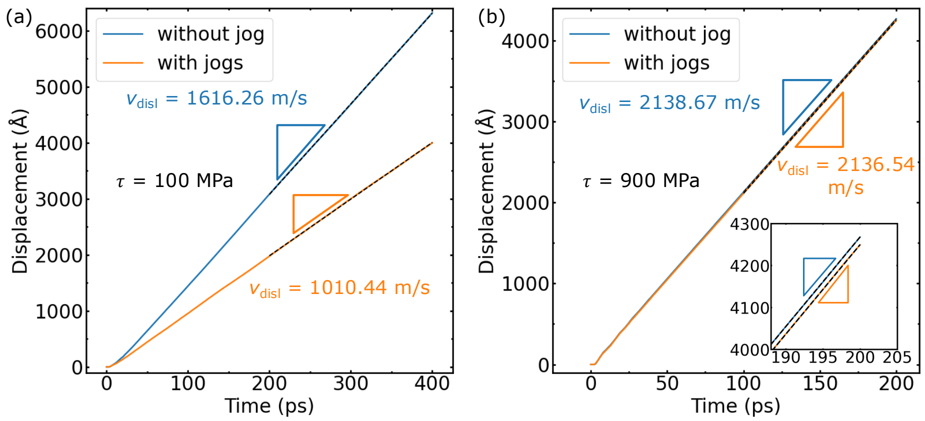


Figure 2: Dislocation displacement as a function of time. Molecular dynamics simulations performed at shear stresses of (a) 100 MPa and (b) 900 MPa. The velocity is determined from the slope of the second half of simulation period, after the dislocation motion has reached a steady-state.

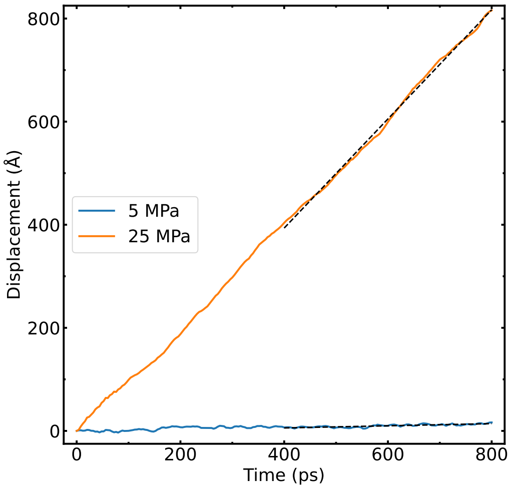


Figure 3: Dislocation displacement as a function of time. Molecular dynamics simulations performed at shear stresses of 5 MPa and 25 MPa. The velocity is determined from the slope of the second half of simulation period.

dislocation-vacancy interaction does not affect the extracted dislocation mobility, we extract the velocity from the time periods both before and after the dislocation encounter the first vacancy it emitted. Fig. 4(a) shows the result for the applied stress of 300 MPa. It can be seen that these two ve-

locities are identical, confirming that the extracted dislocation mobility is not influenced by the dislocation-vacancy interaction. Visualization of the atomic configurations show that the jogged dislocation always just misses the individual vacancies it previous emitted, and all the individual vacancies stay where they are (i.e. do not get re-absorbed by the dislocation) during the simulation.

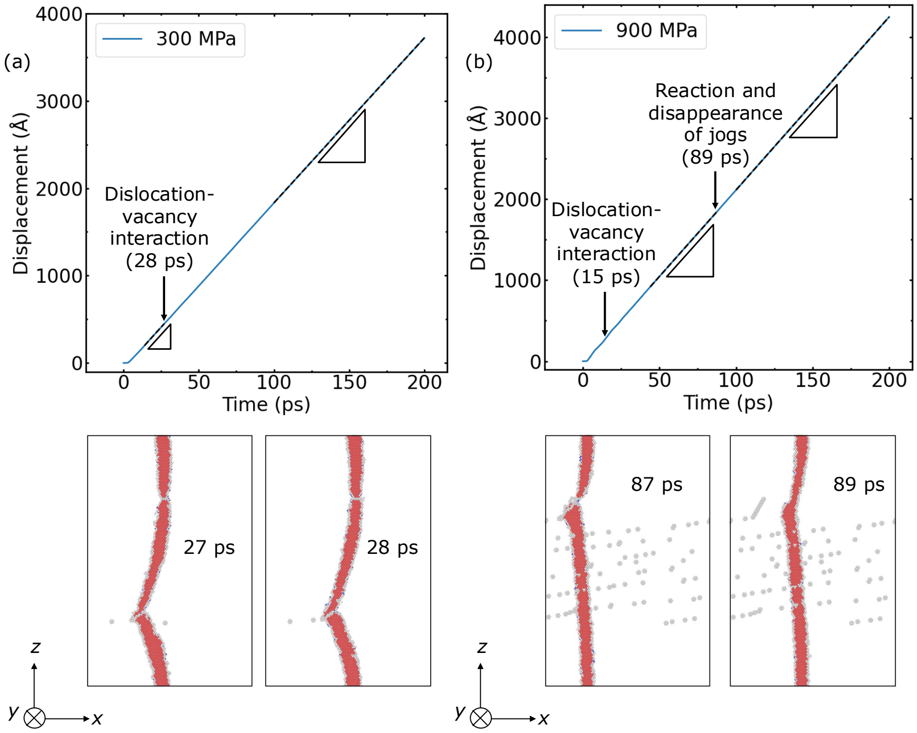


Figure 4: Dislocation displacement as a function of time, together with snapshots of atomic configurations at different times, for molecular dynamics simulations performed at applied shear stresses of (a) 300 MPa and (b) 900 MPa.

For even higher stress at 900 MPa, the constricted jog climbs so much along the dislocation line and gets close to the other (extended) jog after $\sim$ 88 ps. A vacancy cluster is emitted when these two jogs climb to annihilate with each other, as shown in Fig. 4(b). From visualizing the atomic configurations, the dislocation does appear to interact with this vacancy cluster after coming back to its previous location across the periodic boundary. To be safe, the reported dislocation velocity is calculated using data before

the final vacancy cluster is emitted (i.e. time before 88 ps).

## 3. Effect of interatomic potential

To rule out the possibility of artifacts from the interatomic potential used, we re-run the MD simulation at $T = 300\,\mathrm{K}$ and $\tau = 300\,\mathrm{MPa}$ using another EAM potential [1]. Fig. 5 shows that the constricted jog exhibits the same vacancy emission behavior as reported in the main text.

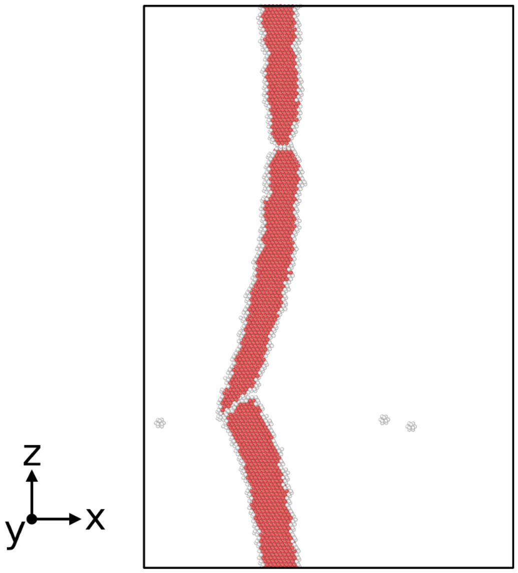


Figure 5: Vacancy emission from jogged dislocation in MD simulations at 300 K and 300 MPa, using EAM potential of Ni from [1].

## References

[1] S. Rao, T. A. Parthasarathy, C. Woodward, Atomistic simulation of cross-slip processes in model fcc structures, Philosophical Magazine A 79 (1999) 1167–1192.
